# Supplementary material for: Building Squares with Optimal State Complexity in Restricted Active Self-Assembly
Source: arXiv:2211.12589 source file (2022-11-22)
Supplement: Supplementary file 1 [file appendix.tex]

\newtheorem*{NoNumTheorem}{Theorem}
\newtheorem*{NoNumCor}{Corollary}

%\subsection{Proof of Theorem \ref{}}\label{app:}
%\begin{NoNumTheorem}
%\end{NoNumTheorem}

\section{Lower Bound Proofs}

\subsection{Proof of Theorem \ref{thm:ndLB}}\label{app:ndLB}
\begin{NoNumTheorem}
For almost all $n$, any Tile Automata system (in particular any Nondeterministic system) that uniquely assembles either a $1\times n$ line or an $n\times n$ square contains $\Omega{(\log^{\frac{1}{4}} n)}$ states.
\end{NoNumTheorem}
\begin{proof} %moved in to paper
We create a one-to-one mapping $b(\Gamma)$ from Nondeterministic TA systems to bit strings.  We use the same mapping as in Theorem~\ref{thm:determ} except for the rule encoding, and now use a $|S|^4$ binary table to specify which rules are, or are not, present in the system.  From Lemma~\ref{lemma:lowerBits},  the minimum state system to build an $n\times n$ square (or $1\times n$ line) has $|S_n|^4 = \Omega(\log n)$ states for almost all $n$, which implies that $|S_n| = \Omega(\log^{\frac{1}{4}} n)$ for almost all $n$.
\end{proof}

\subsection{Proof of Theorem \ref{thm:srLB}}\label{app:srLB}
\begin{NoNumTheorem}
For almost all $n$, any Single-Transition Tile Automata system that uniquely assembles either a $1\times n$ line or an $n\times n$ square contains $\Omega{(\log^{\frac{1}{3}} n)}$ states.
\end{NoNumTheorem}

\begin{proof} %moved in to paper
We use the same bit-string encoding $b(\Gamma)$ as in Theorem~\ref{thm:determ}, except for the encoding of the ruleset, in which we use a $|S|^2\times |S|$ matrix of constants.  The encoding works by encoding the pair of states for a transition in the first column, paired with the second column dictating the state that will change, and the entry in the table denoting which of the two possible states changed.  We thus encode an $|S|$-state system in $O(|S|^3)$ bits, which yields $|S| = \Omega(\log^\frac{1}{3} n)$ for almost all $n$ from Lemma~\ref{lemma:lowerBits}.
\end{proof}

%%%%%%%%%%%%%%%%%%%%%%%%%%%%%%%%%%%%%%%%%%%%%%%%%%%%%%%%%%%%%%%%%%%%%%%%%%%5
\section{String Proofs}

\subsection{Proof of Theorem \ref{thm:2LU}}\label{app:2LU}
\begin{NoNumTheorem}
For any binary string $s$ with length $n > 0$, there exists a freezing tile automata system $\Gamma_s$ with deterministic transition rules, that uniquely assembles an $2 \times (n + 2)$ assembly $A_S$ that represents $S$ with $\mathcal{O}(n^{\frac{1}{2}})$ states %and worst case time $\mathcal{O}(n)$.  
\end{NoNumTheorem}

\begin{proof} %moved in to paper
% States and affinity 
Let $r = n^\frac{1}{2}$. We construct the system $\Gamma_s$ as follows, we use $\BO{r}$ index states and a constant number of seed row and symbol states as described above. Our seed tile is the state $S_A$ and our initial tiles are the $B$ index states, and the two states $a$ and $a'$. Our affinity rules are also described above. Due to affinity strengthening, if one state $\sigma_1$ may transition to another state $\sigma_2$, then $\sigma_1$ must have at least the same affinity rules as $\sigma_2$. This does not cause an issue for the $A$ column as the $a$ state already has affinity with itself so all the $A$ states (besides the states at the top of the column with subscript $A'$) will have vertical affinity with each other. The top tile of each $A$ column does not have affinity with any states on its north and it never gains one by transitioning. For $0 \leq i < r - 1$,  the state $i_B$ has a vertical affinity with $i+1_B$. These $B$ index states transition to symbol states so the symbol states must have vertical affinities with all the $B$ states. 

We encode the starting values of the indexes in the affinity rule of $S_B$ for the $B$ index, and the transition rule between $A$ and $S_A$ for the $A$ column. In the case that the first $B$ state is $r-1_B$ the state that is above $S_A$ will be $a'$. In this case, we transition $a'$ with $S_A$ changing it directly to $0'_A$. 

% Transition Rules
Our transitions rules to build the sections are described above. This system has deterministic rules as each pair of states has up to one transition rule between them. Now, we will formally describe the method to encode our string $S$. 

In Figure \ref{tab:stringLU} we can see $S$ drawn as a table with indices of up to $r$. Let $S( \alpha, \beta  )$ be the $k$th bit of $S$ where $k = \alpha r + \beta - O$. For $\beta < r -1$ we have a transition rules between states $(\alpha_A, \beta_B)$ transitioning to $(\alpha_A, 0i)$ if $S( \alpha, \beta  ) = 0$, or to $(\alpha_A, 1i)$ if $S( \alpha, \beta  ) = 1$. When $\beta = r-1$ we have the same rule but between $(\alpha_A, \beta''_b)$. An overview of these rules can be seen in Figure \ref{fig:indexString}.

% Terminal 
The assembly $A_S$ has the seed row states as its bottom row, followed by rows with a $A$ index state on the left and a symbol state on the right. The top row has the two cap states $N_A$ and $N_B$. This assembly is terminal because none of the initial tiles may attach to the north or south row, the $A$ index states do not have any affinities that allow things to attach on the left, and the symbol states do not allow things to attach on the right. 
We can see this assembly is uniquely produced by viewing how each section is built. The system only has one available move at each step when building the first section until the $A$ column starts indexing. When the $A$ column starts indexing, it will now be able to change the states of the tiles in the $B$ column. We must be careful here, since the affinity strengthening requirement forces our symbol states to have affinity with all the $B$ states. This does not cause an issue for most of the $B$ states as they tiles around them have already attached but this is why the state $r-1_B$ does not transition to a symbol state but instead waits until the next section has started (or the cap row is present) to transition to $r-1''_B$. 
% Run time
%Note that we have a total of $\BO{n}$ tiles in $A_S$ and each tile transitions a constant number of tiles. This means we take a total of $\BO{n}$ steps to build $A_S$ so our run time is upper bounded by $\BO{n}$
\end{proof}

\subsection{Proof of Corollary \ref{col:arbBase}}\label{app:arbBase}
\begin{NoNumCor}
For any base-$b$ string $S$ with length $n > 0$, there exists a freezing tile automata system $\Gamma$ with deterministic transition rules, that uniquely assembles an $(n + 2) \times 2$ assembly which represents $S$ with $\mathcal{O}(n^{\frac{1}{2}} + b)$ states.
\end{NoNumCor}
\begin{proof} %moved in to paper
In order to print base-$b$ strings, we use $b$ index states from $0_S$ to $b-1_S$. We encode the strings in our transitions the same way as the above proof by transitioning the states $(\alpha_A, \beta_B)$ to $(\alpha_A, k_S)$ for $k = S(\alpha, \beta)$.
\end{proof}

\subsection{Proof of Theorem \ref{thm:SRstrings}}\label{app:SRstrings}
\begin{NoNumTheorem}
For any binary string $S$ with length $n > 0$, there exists a Single-Transition tile automata system $\Gamma$, that uniquely assembles an $(2n + 2) \times 3$ assembly which represents $S$ with $\BO{n^\frac{1}{3}}$ states.  
\end{NoNumTheorem}
\begin{proof} %moved in to paper
% Describe state list and verify bound
Let $r = n^\frac{1}{3}$, note that we use $\BO{r}$ index states and look up states in our system. The number of other states is our system is bounded by a constant so the total number of states in $\Gamma$ is  $\BO{n^\frac{1}{3}}$. We use affinity and transition rules to place tiles and index the columns as described above. 

% Describe why it is single rule
Note that the transition rules to index column and the transition rules to signal for another section to build only ever change one of the states involved. The transition rules for the look up do the same as well. Only the $B$ state changes to a look up state. When the look up state transitions with $C$, if they both represent the same index, $C$ transitions to the symbol state of the retrieved bit. If they have different indices, then the look up state transitions to $Bx$. $Bx$ transitions with the index state above it resetting itself. All of these rules only ever change one tile.

As with Theorem \ref{thm:detStringSqrt}, the northmost and southmost rows do not allow other states to attach above/below them, respectively. The states in the $A$ column do not allow tiles to attach on their left. The rightmost column has only $Cu$ and symbol states ($1s$ or $0s$), which do not allow tiles to attach on their right. 

The last column to be indexed in this construction is the $A$ column. Bit gadgets also do not begin to transition until the $A$ state is indexed, so no matter the build order the states that are used will be present before the gadget begins transitioning. Until the $A$ column begins indexing, there is only one step that can take place so we know there are not build orders that result in other terminal assemblies. 
\end{proof}

\subsection{Proof of Theorem \ref{thm:nonDetstrings}}\label{app:nonDetstrings}
\begin{NoNumTheorem}
For any binary string $S$ with length $n > 0$, there exists a tile automata system $\Gamma$, that uniquely assembles an $(2n + 2) \times 4$ assembly which represents $S$ with $\mathcal{O}(n^{\frac{1}{4}} )$ states. 
\end{NoNumTheorem}

\begin{proof} %moved in to paper
Let $r = \lceil n^\frac{1}{4} \rceil$. We use $\BO{r}$ index states to build our bit gadgets. We have $\BO{r}$ look up states and a constant number of pass, fail, and blank states to perform the look up. 

This system uniquely constructs a $(2n + 2) \times 4$ rectangle that represents the string $S$, each bit gadget is a constant height and represents a unique bit of the string. In each bit gadget the test ensure that only the correct bit is retrieved and propagated to the right side of the assembly. By the same argument as the previous constructions this assembly is terminal. A bit gadget does not begin looking up bits until its $A$ column is complete (by transitioning $\beta_B$ to $\beta'_B$) so the system uniquely constructs this rectangle as one move can happen at a time to build the bit gadgets and once a bit gadget is complete it does not affect surrounding tiles as transitions only occur between tiles in the same gadget. 
\end{proof}

%%%%%%%%%%%%%%%%%%%%%%%%%%%%%%%%%%%%%%%%%%%%%%%%%%%%%%%%%%%%%%%%%%%%%%%%%%%5
\section{Rectangle Proofs}

\subsection{Proof of Theorem \ref{thm:DetRect}}\label{app:DetRect}
\begin{NoNumTheorem}
For all $n > 0$, there exists a Deterministic Tile Automata system that uniquely assembles a $\mathcal{O}(\log{n}) \times n$ rectangle using $\mathcal{O}(\log^{\frac{1}{2}}{n})$ states.
\end{NoNumTheorem}
\begin{proof}
% Showing the size of the rectangle is true.
Let assembly $A$ be the $\mathcal{O}(\log{n}) \times n$ rectangle created using the described method.

Breaking down the parts that make up $A$ allow us to analyze the size. The two leftmost columns of $A$ represent the string of size $I_S = \lceil\log{n}\rceil$. We know by Theorem \ref{thm:detStringSqrt} that the height of the string is $I_S + 2$ giving us a height for $A$ of $\BO{\log{n}}$. The rightmost column consists of the stopping column which is full of carry tiles. Based on the binary counter behavior, each column represents a number one less than the column on the right. In order to achieve a length of $n$, we simply need to choose the right starting string to grow $n$ columns. This string would be the binary representation of $2^{\lceil\log{n}\rceil}-n$.

% Showing the number of states
We know from Theorem \ref{thm:detStringSqrt} that the assembly representing the string can be constructed with $\mathcal{O}(n^{\frac{1}{2}})$ states. On top of this a constant number of binary counter states are added, leaving us with $\mathcal{O}(\log^{\frac{1}{2}}{n})$ states for the system that uniquely assembles $A$.

% Showing that A is unique
In order for the system to uniquely assemble $A$, it must always build the same terminal assembly. Height-wise, an attachment of a carry or no carry tile requires the newly placed tile transition before attaching another carry or no carry tile. This prevents the assembly from growing higher than specified since the north row ceases all attachments. Length-wise, the last column  never allows the plus tile to transition into a south tile. This prevents the assembly from growing longer than specified. With these bounds in place, the assembly can grow any way it wants while still being unique. It can grow high, but the north row will prevent it from growing too tall. It can grow long, but each column must first remove their carry before allowing more growth eastward. With the last column being unable to remove any of its carry tiles, the assembly is bounded. Therefore, assembly $A$ is unique.
\end{proof}

\subsection{Proof of Theorem \ref{thm:SRRect}}\label{app:SRRect}
\begin{NoNumTheorem}
For all $n > 0$, there exists a Single-Transition Tile Automata system that uniquely assembles a $\mathcal{O}(\log{n}) \times n$ rectangle using $\Theta(\log^{\frac{1}{3}}{n})$ states.
\end{NoNumTheorem}
\begin{proof}
% Uniqueness should stay the same from 5.1, no need to talk about it

% Showing the size of the rectangle is true.
Building a $\mathcal{O}(\log{n}) \times n$ rectangle follows the same process from Theorem \ref{thm:DetRect}. With a string size of $I_S$, where $I_S= \lceil \log{n} \rceil$, the rectangle will have a height of $\lceil\log{n}\rceil$.

% Showing the number of states
From Theorem \ref{thm:SRstrings} creating a string with a Single-Transition System gives us $\Theta(\log^{\frac{1}{3}}{n})$ states. The bit gadgets in the string have a height of 2. We add a constant amount of states to the binary counter in order to match the height of 2. This leaves us with a constant number of binary counter states resulting in $\Theta(\log^{\frac{1}{3}}{n})$ states to assembly a $\mathcal{O}(\log{n}) \times n$ rectangle.
\end{proof}

\subsection{Proof of Theorem \ref{thm:ntarect}}\label{app:ntarect}
\begin{NoNumTheorem}
For all $n > 0$, there exists a Nondeterministic Tile Automata system that uniquely assembles a $\mathcal{O}(\log{n}) \times n$ rectangle using $\Theta(\log^{\frac{1}{4}}{n})$ states.
\end{NoNumTheorem}
\begin{proof}
% Again, uniqueness should stay the same from 5.1, no need to talk about it
% Showing the size of the rectangle is true.
Similarly to Theorems \ref{thm:DetRect} and \ref{thm:SRRect}, building a $\mathcal{O}(\log{n}) \times n$ rectangle follows the same process. Using a nondeterministic string construction with a string size of $I_S$, where $I_S = \lceil\log{n}\rceil$, the rectangle will have a height of $ \lceil\log{n}\rceil$.

% Showing the number of states
From Theorem \ref{thm:nonDetstrings}, creating a string with nondeterminism gives us $\mathcal{O}(\log^{\frac{1}{4}}{n})$ states. Similar to Theorem \ref{thm:SRRect}, we match the height of the bit gadgets by adding additional states to the binary counter. The binary counter states are constant for any $n > 0$ so the number of states needed to build a rectangle with nondeterminism comes out to $\mathcal{O}(\log^{\frac{1}{4}}{n})$.
\end{proof}

\subsection{Proof of Theorem \ref{thm:varBaseDetRec}} \label{app:varBaseDetRec}

\begin{NoNumTheorem}
For all $n > 0$ there exists a Deterministic Tile Automata system that uniquely assembles a $\mathcal{O}(\frac{\log n}{\log \log n}) \times n$ rectangle using  $\Theta\left((\frac{\log n}{\log \log n})^\frac{1}{2}\right)$ states.
\end{NoNumTheorem}

\begin{proof} %moved to paper
Note that all logarithms shown are base $2$. There are two cases. Case 1: $n \leq 2^{16}$. Let $c$ be the minimum number of states such that for all $w < n' < 2^{16}$, a $w \times n'$ rectangle can be uniquely assembled with $\leq c$ states. We can utilize $c$ states to uniquely assemble a rectangle of the desired size.

Case 2: $n > 2^{16}$. Let $b = \lceil (\frac{\log n}{\log \log n})^\frac{1}{2} \rceil$, and $d = 4 \lceil \frac{ \log n}{\log \log n}\rceil $. We will initialize a variable base counter with value $b^d-n$ represented in base $b$. The binary counter states will then attach to this string, counting up to $b^d$, for a total length of $n$. We will prove that for $n > 2^{16}$ that $b^d \geq n$. Let $b' =  (\frac{\log n}{\log \log n})^\frac{1}{2} $ and $d' =  \frac{ 4\log n}{\log \log n} $.

\begin{align*} 
 \log(b^{d}) &\geq \log(b'^{d'}) \\
 \log(b^{d}) &\geq d' \log(b') \\
\log(b^{d}) &\geq d' \log \left( \left( \frac{d'}{4} \right) ^\frac{1}{2} \right) \\ 
\log(b^{d}) &\geq \frac{d'}{2} \log \left( \frac{d'}{4} \right) \\ 
%\log(b^{d}) & \geq \frac{4}{2}  \frac{ \log n}{\log \log n}  \log \left( \frac{4}{4}  \frac{ \log n}{\log \log n} \right) \\ 
\log(b^{d}) &\geq  \frac{ 2\log n}{\log \log n}  \log \left(  \frac{ \log n}{\log \log n} \right)\\ 
\log(b^{d}) &\geq \frac{ 2\log n}{\log \log n} (\log \log n - \log \log \log n)\\ 
\log(b^{d}) &\geq 2\log n - 2\log n \left( \frac{\log \log \log n}{\log \log n} \right)  \\
\end{align*}

Since $n > 2^{16}$, $\frac{\log \log \log n}{\log \log n} < \frac{1}{2}$.

\begin{align*} 
\log(b^{d}) &\geq 2\log n - 2\log n \left( \frac{1}{2} \right) \\
\log(b^{d}) &\geq \log n\\ 
2^{\log(b^{d})} &\geq 2^{\log n}\\ 
b^d &\geq n 
\end{align*}

By Corollary \ref{cor:varBaseDetStrings} we can create the assembly that represents the necessary $d$-digit base $b$ string  with $d^\frac{1}{2} + b = \Theta\left( (\frac{\log n}{\log \log n})^\frac{1}{2}\right)$ states. The counter which builds off this string requires $\mathcal{O}(b)$ unique states. Therefore for all $n > 0$ we can create a system which uniquely assembles a $\mathcal{O}(\frac{\log n}{\log \log n}) \times n$ rectangle with $\Theta(b) + \Theta(d^{\frac{1}{2}}) + c = \Theta\left( (\frac{\log n}{\log \log n})^\frac{1}{2}\right)$ states.
\end{proof}

%%%%%%%%%%%%%%%%%%%%%%%%%%%%%%%%%%%%%%%%%%%%%%%%%%%%%%%%%%%%%%%%%%%%%%%%%%%5
\section{Square Proofs}

\subsection{Proof of Theorem \ref{thm:detSQ}}\label{app:detSQ}
\begin{NoNumTheorem}
For all $n > 0$, there exists a Tile Automata system with deterministic transition rules that uniquely assembles an $n \times n$ square with $\Theta\left((\frac{\log n}{\log \log n})^\frac{1}{2}\right) states.$
\end{NoNumTheorem}

\begin{proof}
Let $\Gamma_n$ be the deterministic Tile Automata system described above. The width of the rectangle built by $\Gamma_0$ is $n' = n - 4\lceil \frac{\log n}{\log \log n} \rceil - 2$, which is complemented by the $4\lceil \frac{\log n}{\log \log n} \rceil + 2$ width of the next rectangle that is built (that of $\Gamma_1$). This makes the width of the assembly $n$. The same logic shows the height of the assembly is $n$.

This system includes all states from $\Gamma_0,\Gamma_1,\Gamma_2,$ and $\Gamma_3$. By Theorem \ref{thm:varBaseDetRec}, each of these systems can be created with $(\frac{\log n}{\log \log n})^\frac{1}{2}$ states. On top of this, a constant number of states are added to $\Gamma_n$ to allow for the reseeding and filling functionality described above. Therefore $\Gamma_n$ requires $\Theta\left((\frac{\log n}{\log \log n})^\frac{1}{2}\right)$ states.
\end{proof}

\subsection{Proof of Theorem \ref{thm:srSQ}}\label{app:srSQ}
\begin{NoNumTheorem}
For all $n > 0$, there exists a Single-Transition Tile Automata system that uniquely assembles an $n \times n$ square with $\Theta(\log ^\frac{1}{3} n)$ states.
\end{NoNumTheorem}
\begin{proof}
The proof follows the same logic, with the only difference being the process for constructing the rectangles. Let $n' = n - 2\lceil \log n \rceil - 4$. Theorem \ref{thm:SRRect} states that a length $n'$ rectangle can be uniquely assembled by a system with $\Theta(\log^\frac{1}{3}n)$ states. Let $\Gamma_0,\Gamma_1,\Gamma_2, \Gamma_3$ be four of these systems with the same modifications previously described. We combine these to create $\Gamma_n$. From Theorem \ref{thm:SRstrings}, building the length $\lceil \log n \rceil$ string requires building an assembly of size $3 \times \lceil 2\log n \rceil + 2$. Therefore the shorter dimension of each rectangle will be $\lceil 2\log n + 4 \rceil$. When the rectangles are consecutively built in the same arrangment as before, an $n\times n$ assembly is created. Since each system $\Gamma_0,\ldots,\Gamma_3$ requires $\Theta(\log^\frac{1}{3}n)$ states, and a constant number of states was added in the creation of $\Gamma_n$, $\Gamma_n$ requires $\Theta(\log^\frac{1}{3}n)$ states.
\end{proof}

\subsection{Proof of Theorem \ref{thm:ndSQ}}\label{app:ndSQ}
\begin{NoNumTheorem}
For all $n > 0$, there exists a Tile Automata system that uniquely assembles an $n \times n$ square with $\Theta(\log ^\frac{1}{4} n)$ states.
\end{NoNumTheorem}
\begin{proof}
By Theorem \ref{thm:nonDetstrings} we can create a system which uniquely assembles a length $n' = n - ((2n + 2) \times 4)$ rectangle with $\Theta(\log ^\frac{1}{4} n)$ states. These rectangles will have width $(2n + 2) \times 4$. Using the same technique we can create a system $\Gamma_n$ which uniquely assembles an $n \times n$ square with $\Theta(\log ^\frac{1}{4} n)$ states.
\end{proof}
